# Supplementary material for: Towards better understanding of gradient-based attribution methods for Deep Neural Networks
Source: arXiv:1711.06104 source file (2018-03-07)
Supplement: Supplementary file 1 [file additional.tex]

%Gradient * Input, being based on the instant gradient at the network input, satisfies Implementation Invariance but does not satisfy the properties of Sensitivity and Completeness\citep{sundararajan17a}. The problem with Sensitivity is that the instant gradient can be zero due to saturation of the nonlinearities even for those features that have strong marginal contribution. In other words, an input feature might have a strong global effect but small local derivative. We notice also multiplying the input with the gradient is necessary for this to be a \textit{global} attribution method. In fact, if the instant gradient approximates the average gradient (ie. if the function of interest is linear) then Gradient * Input matches Integrated Gradients.

%Contrarily, the Saliency method only uses the (absolute) gradient. This implies that the method can only describe the network locally unless we assume the network is nearly linear. By taking the absolute value of the gradient, the attributions generated by Saliency only provide information about which features can be changed the least in order for the output to change the most but loosing the direction of the expected change. This method is therefore a \textit{local} method and as such cannot satisfy Sensitivity and Completeness. Being gradient-based, it does however satisfy Implementation Invariance.


%The function $g(z_j) = f(z_j) / (z_j + \epsilon)$ used by LRP can be seen as the average gradient of $f$ between $0$ and the value $z_j$, assuming that $f(0) = 0$, condition that is only verified for nonlinearities that passes through the origin (ie. ReLU and Tanh). We speculate this is the reason why LRP performs poorly when this condition is not met, as visible in Figure \ref{fig:act_comparison}. With Sigmoid and Tanh nonlinearities, $g(z_i) < 0$ for $z_i < 0$. When this happens, all attributions are inverted in sign causing the attribution method to fail to provide meaningful results. Given this assumption that the attributions should never flip their sign when passing though a nonlinearity, the role of $\epsilon$ in the original LRP formulation becomes more clear, not only to avoid numerical instabilities but also to avoid a catastrophic inversion of sign.




%\caption{Comparison of five gradient-based attribution methods together with the perturbation method by Zeiler \textit{et al.} performed pixel-wise on a CNN trained with four different nonlinearities on the MNIST dataset \citep{lecun1998mnist}. The input to the network are 28x28 images where the foreground has value 1 and the background value -1. Red areas indicate positive attribution for the correct class ("zero"), while blue indicates negative attribution. While the test classification accuracy with the different nonlinearities is comparable, the attribution heatmaps differ. For example with a network trained with Sigmoid, Integrated Gradients and DeepLIFT assign greater importance to missing pixels in the middle of the image than with networks trained with Relu or Softplus. According to all methods, the attributions using Tanh are less sparse than with other activations. Notice how LRP* fails to generate meaningful attributions with Sigmoid and Softplus. Best seen in electronic form.}


%Here, we suggest that a desirable property of an attribution method is the ability to \textit{rank} subsets of features from a given sample according to their influence on the output. In this context by "influence" we mean the variation of a target output when the network under analysis is stimulated with the original input and with an input where some features have been removed, in the sense discussed in Subsection \ref{sec:perturbation} and in Appendix \ref{sec:baseline}.


%Moreover, we argue that the current formulation for the attribution problem is inherently ambiguous for nonlinear systems. Consider a network that implements the function $f(x_1, x_2) = x_1 + x_2 + 2 \cdot ReLU(x_1 - x_2) + 2 \cdot ReLU(x_2 - x_1)$. We want to find attributions for the input $(x_1, x_2) = (1,1)$. If we remove either one of the features the output \textit{increases}, from $2$ to $3$. On the contrary, if we remove both features the output \textit{decreases}, form $2$ to $0$. Given this observation, attributions that could explain the system overall can not exist. Instead, one could look for attributions explaining the influence of single features or the influence of both features considered together. In fact, the methods analyzed in the previous section would give different results: Occlusion-1 method would assign a relevance of $-1$ to both units, while all gradient-based methods would assign both units a score of $1$. We believe there is no reason to consider one solution better than the other, unless the problem is further defined.




%Quantitative metrics have been proposed in the past, but these can be subject to different kind of biases as well. For example, the \textit{sparsity} of attribution maps \citep{samek2016evaluating} is a metric biased by the humans' preference for simple explanations. Another metric often used is sequential feature deletion  \citep{samek2016evaluating}: in this case a significant portion of the input features (eg. 10\%) are sequentially replaced with a baseline value, while the change of the target output is recorded at every iteration. The order of removal is the rank of the features based on the attribution score, where the feature with highest attribution is removed first.  An ordering of features such that the most sensitive ones are ranked first is expected to produce a steep decrease of the measured output. We notice, however, that this only allows to reveal those methods that are better in detecting the aggregate effect of a group of features together. 
